# Supplementary material for: Syntax-Aware On-the-Fly Code Completion
Source: arXiv:2211.04673 source file (2023-05-01)
Supplement: Supplementary file 1 [file appendix.tex]

\revise{R3.12}{
\section{\our-IFN Analysis}
\our-IFN is finetuned separately on the supporting task (token type prediction) and then the target task (code token prediction). 
Table~\ref{tab:rq2} shows \our-IFN performance is in second place.
However, we observed the token type accuracy in token-level prediction and found that the accuracy of \our-IFN goes down to 0\%.
As a result, it shows that the model faces prevalent problems when training a model sequentially: a catastrophic forgetting~\cite{mccloskey1989catastrophic, kaushik2021understanding}.
In other words, \our-IFN has already forgotten the token type information which might be the reason for the worse results than \our-Hard which can access the type data throughout the training. Although our main focus is on the performance of the code prediction task, we note this result in the discussion for a better understanding.

% Additionally, we also show the accuracy of token-level prediction for token types in Table.~\ref{tab:rq2} which clearly emphasizes the difference between MTL and IFN. 
% Even though the results of the IFN model for code completion are comparable to the one produced by the hard parameters sharing model with a difference of 0.63\% (from 76.52\% to 77.00\%) in the token-level prediction accuracy and 1.88\% (from 42.04\% to 42.83\%) in the line-level prediction exact match, we can observe that the IFN \emph{type} prediction accuracy goes down to 0\%.
% As the IFN model is fine-tuned firstly on type prediction (supporting task), then fine-tuned on code prediction (target task); thus, this could cause the prevalent problems when training a model sequentially: a catastrophic forgetting~\cite{mccloskey1989catastrophic, kaushik2021understanding}.
% As a result, the IFN model has already forgotten the token type information which is the reason for the worse results than the hard parameters sharing model that can access the supporting data all along the training.
}
